# Supplementary material for: Irregular Oscillatory-Patterns in the Early-Time Region of Coherent Phonon Generation in Silicon
Source: arXiv:1705.07257 ancillary file (2017-05-20)
Supplement: Supplementary file 1 [file SupplementalMaterial.pdf]

## Theoretical Framework

Supplemental Material provides the detail of the theoretical framework constructed for the present study. Section I gives the Hamiltonian of the system concerned, followed by the equations of motion of polaronic quasiparticle (PQ) operators in Sec. II, and the retarded phonon Green function and coherent phonon (CP) displacement function in Sec. III. This also includes two appendices. Atomic units are used throughout.

### I. THE HAMILTONIAN OF THE SYSTEM CONCERNED

The total Hamiltonian of the present system is provided by $\hat{H} = \hat{H}_e + \hat{H}'(t) + \hat{H}_p + \hat{H}_{e-p}$, where

$$\begin{aligned}\hat{H}_e &= \sum_{b\boldsymbol{k}} \varepsilon_{b\boldsymbol{k}} a^\dagger_{b\boldsymbol{k}} a_{b\boldsymbol{k}} + \frac{1}{2}\sum_{\boldsymbol{q}\neq 0} V^{(C)}_{\boldsymbol{q}} \\ &\times \sum_{bb'\boldsymbol{k}\boldsymbol{k}'} a^\dagger_{b\boldsymbol{k}+\boldsymbol{q}} a^\dagger_{b'\boldsymbol{k}'-\boldsymbol{q}} a_{b'\boldsymbol{k}'} a_{b\boldsymbol{k}}, \end{aligned} \tag{1}$$

$$\hat{H}'(t) = -\sum_{\boldsymbol{k}} \left[\Omega_{cv}(t)\, a^\dagger_{c\boldsymbol{k}} a_{v\boldsymbol{k}} + \Omega_{vc}(t)\, a^\dagger_{v\boldsymbol{k}} a_{c\boldsymbol{k}}\right], \tag{2}$$

$$\hat{H}_p = \sum_{\boldsymbol{q}} \omega_{\boldsymbol{q}ph} c^\dagger_{\boldsymbol{q}} c_{\boldsymbol{q}}, \tag{3}$$

and

$$\hat{H}_{e-p} = \sum_{b,\boldsymbol{q},\boldsymbol{k}} \left(g_{b\boldsymbol{q}} c_{\boldsymbol{q}} a^\dagger_{b\boldsymbol{k}+\boldsymbol{q}} a_{b\boldsymbol{k}} + g^*_{b\boldsymbol{q}} c^\dagger_{\boldsymbol{q}} a^\dagger_{b\boldsymbol{k}} a_{b\boldsymbol{k}+\boldsymbol{q}}\right). \tag{4}$$

$\hat{H}_e$ is a two-band electron Hamiltonian, and $\hat{H}'(t)$ is the electron-light interaction at time $t$. Here, $a^\dagger_{b\boldsymbol{k}}$ and $a_{b\boldsymbol{k}}$ are creation and annihilation operators of electron with Bloch momentum $\boldsymbol{k}$ in band $b$, respectively; $b = c$ for the conduction band, and $b = v$ for the valence band. $\varepsilon_{b\boldsymbol{k}}$ is an energy dispersion of $b$-band electron. $V^{(C)}_{\boldsymbol{q}}$ is a Coulomb potential represented as

$$V^{(C)}_{\boldsymbol{q}} = \frac{4\pi}{\epsilon_\infty V}\frac{1}{\boldsymbol{q}^2}, \tag{5}$$

where $\boldsymbol{q}$, $V$, and $\epsilon_\infty$ are momentum, volume of crystal, and a dielectric constant in the high-frequency limit, respectively. Rabi frequency $\Omega_{b\bar{b}}(t)$ relevant to a pump laser is given by [1]

$$\Omega_{b\bar{b}}(t) = \Omega_{0b\bar{b}} \cos(\omega_0 t + \delta) f(t), \tag{6}$$

where $\Omega_{0b\bar{b}}$ is the product of an electric dipole moment between $b$ and $\bar{b}$-bands and the peak amplitude of the laser field. The barred index $\bar{b}$ means that this is unequal to $b$, namely, $\bar{c} = v$ and $\bar{v} = c$. Further, the laser parameters of $\omega_0$, $f(t)$, and $\delta$ are a center frequency, a pulse-envelope function, and a carrier-envelope phase (CEP), respectively. $f(t)$ is set to the Gaussian function, that is, $f(t) = \exp(-t^2/2\sigma^2)$, with temporal width (FWHM) $\tau_L$ given by $\tau_L = 2\sqrt{2\ln 2}\sigma$. $\hat{H}_p$ is an LO-phonon Hamiltonian and $\hat{H}_{e-p}$ is an electron-phonon interaction, where $c^\dagger_{\boldsymbol{q}}$ and $c_{\boldsymbol{q}}$ are creation and annihilation operators of LO-phonon with energy dispersion $\omega_{\boldsymbol{q}ph}$, respectively, where the zero-point energy of the phonon is omitted just for the sake of simplicity. $g_{b\boldsymbol{q}}$ is a coupling constant of a $b$-band electron with the LO-phonon.

### II. EQUATIONS OF MOTION OF POLARONIC QUASIPARTICLE OPERATORS

We consider a composite operator defined by $A^\dagger_{\boldsymbol{q}}(\boldsymbol{k}bb') = a^\dagger_{b\boldsymbol{k}+\boldsymbol{q}} a_{b'\boldsymbol{k}}$, which represents an induced carrier density matrix with anisotropic momentum $\boldsymbol{q}$; the magnitude of it is quite small, but finite ($\boldsymbol{q} \neq 0$) [2]. As outlined in Appendix A, a collective excitation mode — a plasmon — is represented as the following operator:

$$B^\dagger_{\boldsymbol{q}} = \sum_{\boldsymbol{k}b} A^\dagger_{\boldsymbol{q}}(\boldsymbol{k}bb) U^R_{\boldsymbol{q}}(\boldsymbol{k}bb) \tag{7}$$

in terms of the intraband density matrix $A^\dagger_{\boldsymbol{q}}(\boldsymbol{k}bb)$ with time $t$ fixed as an adiabatic parameter, where $U^R_{\boldsymbol{q}}(\boldsymbol{k}bb)$ is given by Eq. (A5).

The equations of motion of $B^\dagger_{\boldsymbol{q}}$, $c^\dagger_{\boldsymbol{q}}$, and the interband density matrix $A^\dagger_{\boldsymbol{q}}(\boldsymbol{k}b\bar{b})$ associated with an individual excitation mode are provided in terms of the Heisenberg equation as

$$\begin{aligned}-i\frac{dB^\dagger_{\boldsymbol{q}}}{dt} &= \bar{\omega}_{\boldsymbol{q}pl} B^\dagger_{\boldsymbol{q}} + M^*_{\boldsymbol{q}pl} c^\dagger_{\boldsymbol{q}} + M_{-\boldsymbol{q}pl} c_{-\boldsymbol{q}} \\ &+ \sum_{\boldsymbol{k}} \Omega^{(R)}_{b\bar{b}\boldsymbol{k}}(t) \left\{U^R_{\boldsymbol{q}}(\boldsymbol{k}bb) - U^R_{\boldsymbol{q}}(\boldsymbol{k}\bar{b}\bar{b})\right\} \\ &\times A^\dagger_{\boldsymbol{q}}(\boldsymbol{k}b\bar{b}), \end{aligned} \tag{8}$$

$$-i\frac{dc^\dagger_{\boldsymbol{q}}}{dt} = \bar{\omega}_{\boldsymbol{q}ph} c^\dagger_{\boldsymbol{q}} + M_{\boldsymbol{q}pl} B^\dagger_{\boldsymbol{q}}, \tag{9}$$

and

$$\begin{aligned}-i\frac{dA^\dagger_{\boldsymbol{q}}(\boldsymbol{k}b\bar{b})}{dt} &= (\omega_{b\bar{b}\boldsymbol{k}\boldsymbol{q}} + i\gamma_{b\bar{b}\boldsymbol{k}\boldsymbol{q}}) A^\dagger_{\boldsymbol{q}}(\boldsymbol{k}b\bar{b}) \\ &+ [\Omega^{(R)}_{\bar{b}b\boldsymbol{k}}(t) \left\{U^{L\dagger}_{\boldsymbol{q}}(\boldsymbol{k}bb) - U^{L\dagger}_{\boldsymbol{q}}(\boldsymbol{k}\bar{b}\bar{b})\right\} \\ &+ V^{(C)}_{\boldsymbol{q}} N^L_{\boldsymbol{q}} (\rho_{b\bar{b}\boldsymbol{k}} - \rho_{b\bar{b}\boldsymbol{k}+\boldsymbol{q}})] B^\dagger_{\boldsymbol{q}}, \end{aligned} \tag{10}$$

respectively, where $\bar{\omega}_{\boldsymbol{q}pl} = \omega_{\boldsymbol{q}pl} - iW_{\boldsymbol{q}} + i\gamma_{\boldsymbol{q}pl}$ and $\bar{\omega}_{\boldsymbol{q}ph} = \omega_{\boldsymbol{q}} + i\gamma_{\boldsymbol{q}ph}$ with $\gamma_{\boldsymbol{q}pl}$, $\gamma_{\boldsymbol{q}ph}$, and $\gamma_{b\bar{b}\boldsymbol{k}\boldsymbol{q}}$ as phenomenological damping constants of phonon, plasmon, and individual excitation mode, respectively. Moreover, $\omega_{bb'\boldsymbol{k}\boldsymbol{q}} = \varepsilon^{(r)}_{b\boldsymbol{k}+\boldsymbol{q}} - \varepsilon^{(r)}_{b'\boldsymbol{k}}$, where $\varepsilon^{(r)}_{b\boldsymbol{k}} = \varepsilon_{b\boldsymbol{k}} - \sum_{\boldsymbol{q}} V^{(C)}_{\boldsymbol{q}} \rho_{bb\boldsymbol{k}+\boldsymbol{q}}$, which represents a renormalized $b$-band electron energy, with $\rho_{bb'\boldsymbol{k}} \equiv \langle a^\dagger_{b\boldsymbol{k}} a_{b'\boldsymbol{k}}\rangle$ as a single-particle density matrix; $\langle \hat{X}\rangle$ represents an expectation value of operator $\hat{X}$ with

respect to the ground state. The plasma frequency $\omega_{\boldsymbol{q}pl}$ and $U_{\boldsymbol{q}}^{L\dagger}(\boldsymbol{k}bb)$ associated with $U_{\boldsymbol{q}}^{R}(\boldsymbol{k}bb)$ are given by Eqs. (A3) and (A4), respectively. An effective coupling constant between the plasmon and the LO-phonon is given by [2]

$$M_{\boldsymbol{q}pl} = \sum_{\boldsymbol{k}b} g_{b\boldsymbol{q}} U_{\boldsymbol{q}}^{L\dagger}(\boldsymbol{k}bb). \tag{11}$$

In addition, $N_{\boldsymbol{q}}^{L} = \sum_{\boldsymbol{k}b} U_{\boldsymbol{q}}^{L\dagger}(\boldsymbol{k}bb)$, $W_{\boldsymbol{q}} = \sum_{\boldsymbol{k}b} U_{\boldsymbol{q}}^{L\dagger}(\boldsymbol{k}bb)\left[dU_{\boldsymbol{q}}^{R}(\boldsymbol{k}bb)/dt\right]$, which represents a non-adiabatic coupling, and

$$\Omega_{b\bar{b}\boldsymbol{k}}^{(R)}(t) = \Omega_{b\bar{b}}(t) + \sum_{\boldsymbol{q}} V_{\boldsymbol{q}}^{(C)} \rho_{b\bar{b}\boldsymbol{k}+\boldsymbol{q}}. \tag{12}$$

Furthermore, the rotating wave approximation [3] is employed in order to remove high-frequency contributions from Eqs. (8) and (10); $A_{\boldsymbol{q}}^{\dagger}(\boldsymbol{k}b\bar{b})$ and $\rho_{b\bar{b}\boldsymbol{k}}$ are replaced by $e^{i\bar{\omega}_{b\bar{b}}t}\bar{A}_{\boldsymbol{q}}^{\dagger}(\boldsymbol{k}b\bar{b})$ and $e^{i\bar{\omega}_{b\bar{b}}t}\bar{\rho}_{b\bar{b}\boldsymbol{k}}$, respectively, where $\bar{\omega}_{cv} = \omega_0$ and $\bar{\omega}_{vc} = -\omega_0$. Thus, Eqs. (8) and (10) are recast into

$$-i\frac{dB_{\boldsymbol{q}}^{\dagger}}{dt} = \bar{\omega}_{\boldsymbol{q}pl}B_{\boldsymbol{q}}^{\dagger} + M_{\boldsymbol{q}pl}^{*}c_{\boldsymbol{q}}^{\dagger} + \sum_{\boldsymbol{k}b} M_{\boldsymbol{q}}'(\boldsymbol{k}b\bar{b})\bar{A}_{\boldsymbol{q}}^{\dagger}(\boldsymbol{k}b\bar{b}), \tag{13}$$

and

$$-i\frac{d\bar{A}_{\boldsymbol{q}}^{\dagger}(\boldsymbol{k}b\bar{b})}{dt} = \bar{\omega}_{b\bar{b}\boldsymbol{k}\boldsymbol{q}}\bar{A}_{\boldsymbol{q}}^{\dagger}(\boldsymbol{k}b\bar{b}) + M_{\boldsymbol{q}}(\boldsymbol{k}b\bar{b})B_{\boldsymbol{q}}^{\dagger}, \tag{14}$$

respectively, where

$$\bar{\omega}_{b\bar{b}\boldsymbol{k}\boldsymbol{q}} = \omega_{b\bar{b}\boldsymbol{k}\boldsymbol{q}} - \bar{\omega}_{b\bar{b}} + i\gamma_{b\bar{b}\boldsymbol{k}\boldsymbol{q}}, \tag{15}$$

$$\begin{aligned} M_{\boldsymbol{q}}(\boldsymbol{k}b\bar{b}) &= \bar{\Omega}_{\bar{b}b\boldsymbol{k}}^{(R)}(t)\left\{U_{\boldsymbol{q}}^{L\dagger}(\boldsymbol{k}bb) - U_{\boldsymbol{q}}^{L\dagger}(\boldsymbol{k}\bar{b}\bar{b})\right\} \\ &\quad + V_{\boldsymbol{q}}^{(C)}N_{\boldsymbol{q}}^{L}(\bar{\rho}_{b\bar{b}\boldsymbol{k}} - \bar{\rho}_{b\bar{b}\boldsymbol{k}+\boldsymbol{q}}), \end{aligned} \tag{16}$$

and

$$M_{\boldsymbol{q}}'(\boldsymbol{k}b\bar{b}) = \bar{\Omega}_{b\bar{b}\boldsymbol{k}}^{(R)}(t)\left\{U_{\boldsymbol{q}}^{R}(\boldsymbol{k}bb) - U_{\boldsymbol{q}}^{R}(\boldsymbol{k}\bar{b}\bar{b})\right\}. \tag{17}$$

where

$$\bar{\Omega}_{b\bar{b}\boldsymbol{k}}^{(R)}(t) = \frac{1}{2}\Omega_{0b\bar{b}}f(t)\exp(-i\bar{\delta}_{b\bar{b}}) + \sum_{\boldsymbol{q}} V_{\boldsymbol{q}}^{(C)}\bar{\rho}_{b\bar{b}\boldsymbol{k}+\boldsymbol{q}}, \tag{18}$$

with $\bar{\delta}_{cv} = \delta$ and $\bar{\delta}_{vc} = -\delta$. In addition, an effect of $M_{-\boldsymbol{q}pl}$ of Eq. (8) is neglected [2].

Equations (9), (13), and (14) are integrated into a single equation as follows;

$$-i\left[c_{\boldsymbol{q}}^{\dagger}, \bar{A}_{\boldsymbol{q}}^{\dagger}(\boldsymbol{k}b\bar{b})\cdots, B_{\boldsymbol{q}}^{\dagger}\right] = \left[c_{\boldsymbol{q}}^{\dagger}, \bar{A}_{\boldsymbol{q}}^{\dagger}(\boldsymbol{k}b\bar{b})\cdots, B_{\boldsymbol{q}}^{\dagger}\right]\bar{Z}_{\boldsymbol{q}}, \tag{19}$$

where the vector notation $\left[c_{\boldsymbol{q}}^{\dagger}, \bar{A}_{\boldsymbol{q}}^{\dagger}(\boldsymbol{k}b\bar{b})\cdots, B_{\boldsymbol{q}}^{\dagger}\right]$ is used, and the non-Hermitian matrix $\bar{Z}_{\boldsymbol{q}}$ is given by

$$\bar{Z}_{\boldsymbol{q}} = \begin{bmatrix} \bar{\omega}_{\boldsymbol{q}ph} & 0 & 0 & M_{\boldsymbol{q}pl}^{*} \\ 0 & \bar{\omega}_{b\bar{b}\boldsymbol{k}\boldsymbol{q}} & 0 & M_{\boldsymbol{q}}'(\boldsymbol{k}b\bar{b}) \\ 0 & 0 & \ddots & \vdots \\ M_{\boldsymbol{q}pl} & M_{\boldsymbol{q}}(\boldsymbol{k}b\bar{b}) & \cdots & \bar{\omega}_{\boldsymbol{q}pl} \end{bmatrix}. \tag{20}$$

Here, the indices of $ph$, $pl$, and $(\boldsymbol{k}b\bar{b})$ are introduced to represent a phonon, a plasmon, and interband carrier density, respectively.

As described in Appendix B, we solve the left and right eigenvalue problems [4] of $\bar{Z}_{\boldsymbol{q}}$ as $V_{\boldsymbol{q}i}^{L\dagger}\bar{Z}_{\boldsymbol{q}} = E_{\boldsymbol{q}i}V_{\boldsymbol{q}i}^{L\dagger}$ and $\bar{Z}_{\boldsymbol{q}}V_{\boldsymbol{q}i}^{R} = V_{\boldsymbol{q}i}^{R}E_{\boldsymbol{q}i}$, respectively, where $E_{\boldsymbol{q}i}$ ($i = \{ph, (\boldsymbol{k}b\bar{b})\cdots, pl\}$) represents the $i$th eigenvalue, and $V_{\boldsymbol{q}i}^{L}$ and $V_{\boldsymbol{q}i}^{R}$ represent the associated biorthogonal set of eigenvectors. Now, the PQ operator defined as

$$P_{\boldsymbol{q}i}^{\dagger} = \left[c_{\boldsymbol{q}}^{\dagger}, \bar{A}_{\boldsymbol{q}}^{\dagger}(\boldsymbol{k}b\bar{b})\cdots, B_{\boldsymbol{q}}^{\dagger}\right]V_{\boldsymbol{q}i}^{R} \tag{21}$$

is introduced. Thus, Eqs. (9), (13), and (14) are recast into a single equation of motion of $P_{\boldsymbol{q}i}^{\dagger}$ given by

$$-i\frac{dP_{\boldsymbol{q}i}^{\dagger}}{dt} = E_{\boldsymbol{q}i}P_{\boldsymbol{q}i}^{\dagger} - i\sum_{i'} P_{\boldsymbol{q}i'}^{\dagger}X_{\boldsymbol{q}i'i}, \tag{22}$$

where a non-adiabatic coupling between $i$ and $i'$ is represented as

$$X_{\boldsymbol{q}ii'} = \sum_{i''} V_{\boldsymbol{q}ii''}^{L\dagger}\frac{dV_{\boldsymbol{q}i''i'}^{R}}{dt} \equiv V_{\boldsymbol{q}i}^{L\dagger}\frac{dV_{\boldsymbol{q}i'}^{R}}{dt}. \tag{23}$$

Due to the Hellman-Feynman theorem, this is rewritten as

$$X_{\boldsymbol{q}ii'} = \frac{V_{\boldsymbol{q}i}^{L\dagger}\frac{d\bar{Z}_{\boldsymbol{q}}}{dt}V_{\boldsymbol{q}i'}^{R}}{E_{\boldsymbol{q}i'} - E_{\boldsymbol{q}i}},\ i \neq i', \tag{24}$$

and $X_{\boldsymbol{q}ii} \neq 0$.

## III. RETARDED PHONON GREEN FUNCTION AND CP DISPLACEMENT FUNCTION

A retarded phonon Green function $D_{\boldsymbol{q}}^{R}(t,t')$ is given by [2, 5]

$$D_{\boldsymbol{q}}^{R}(t,t') = \bar{D}_{\boldsymbol{q}}^{R}(t,t') + \left[\bar{D}_{-\boldsymbol{q}}^{R}(t,t')\right]^{*}, \tag{25}$$

where

$$\begin{aligned} \bar{D}_{\boldsymbol{q}}^{R}(t,t') &= -i\left\langle\left[c_{\boldsymbol{q}}(t), c_{\boldsymbol{q}}^{\dagger}(t')\right]\right\rangle\theta(t-t') \\ &= -i\sum_{ii'} V_{\boldsymbol{q}phi}^{L}(t)\left\langle\left[P_{\boldsymbol{q}i}(t), P_{\boldsymbol{q}i'}^{\dagger}(t')\right]\right\rangle \\ &\quad \times V_{\boldsymbol{q}i'ph}^{L\dagger}(t')\theta(t-t'), \end{aligned} \tag{26}$$

and $\bar{D}_{-\boldsymbol{q}}^{R}(t,t') = \bar{D}_{\boldsymbol{q}}^{R}(t,t')$. Here, $c_{\boldsymbol{q}}^{\dagger}$ is represented in terms of the PQ operator as $c_{\boldsymbol{q}}^{\dagger} = \sum_i P_{\boldsymbol{q}i}^{\dagger}V_{\boldsymbol{q}iph}^{L\dagger}$ using Eq. (21). In the linear response theory, $D_{\boldsymbol{q}}^{R}(t,t')$ indicates an induced charge density of ionic-core introduced by a weak external-potential at time $t'$ that is delta-shaped, namely, in proportion to $\delta(t')$.

Equation (22) can be approximately solved by neglecting the contribution from the non-adiabatic coupling of

the second term in the right-hand side; in other words, the adiabatic approximation is employed here [2]. Thus, Eq. (26) becomes

$$\bar{D}^R_{\boldsymbol{q}}(t,t') \approx -i\sum_{jj'} V^L_{\boldsymbol{q}ph,j}(t)\,\exp\left[-i\int_{-\infty}^{t} dt'' E^*_{\boldsymbol{q}j}(t'')\right] \times \left\langle \left[P_{\boldsymbol{q}j}(-\infty), P^\dagger_{\boldsymbol{q}j'}(-\infty)\right]\right\rangle \theta(t-t') \times \exp\left[+i\int_{-\infty}^{t'} dt'' E_{\boldsymbol{q}j'}(t'')\right] V^{L\dagger}_{\boldsymbol{q}j',ph}(t'). \quad (27)$$

In the case of an undoped semiconductor, the term of $\langle [P_{\boldsymbol{q}j}(-\infty), P^\dagger_{\boldsymbol{q}j'}(-\infty)]\rangle$ is given by

$$\left\langle \left[P_{\boldsymbol{q}j}(-\infty), P^\dagger_{\boldsymbol{q}j'}(-\infty)\right]\right\rangle = \delta_{j,ph}\delta_{jj'}, \quad (28)$$

where the following relations are used: $V^{R\dagger}_{\boldsymbol{q}ph,j}(-\infty) = \delta_{ph,j}$, $\left[c_{\boldsymbol{q}}(-\infty), c^\dagger_{\boldsymbol{q}}(-\infty)\right] = 1$, and $\left[c_{\boldsymbol{q}}(-\infty), B^\dagger_{\boldsymbol{q}}(-\infty)\right] = \left[c_{\boldsymbol{q}}(-\infty), A^\dagger_{\boldsymbol{q}}(\boldsymbol{k}b\bar{b})\big(-\infty)\right] = 0$. Therefore, Eq. (27) is rewritten as

$$\bar{D}^R_{\boldsymbol{q}}(t,t') = -ie^{-i\omega_{\boldsymbol{q}ph}(t-t')}\xi_{\boldsymbol{q}}(t,t') \times V^L_{\boldsymbol{q}phph}(t)V^{L\dagger}_{\boldsymbol{q}phph}(t')\theta(t-t'), \quad (29)$$

where

$$\xi_{\boldsymbol{q}}(t,t') = \exp\left[-\int_{-\infty}^{t} dt''\,\mathrm{Im}E_{\boldsymbol{q}ph}(t'')\right] \times \exp\left[-i\int_{t'}^{t} dt''\left\{\mathrm{Re}E_{\boldsymbol{q}ph}(t'') - \omega_{\boldsymbol{q}ph}\right\}\right] \times \exp\left[-\int_{-\infty}^{t'} dt''\,\mathrm{Im}E_{\boldsymbol{q}ph}(t'')\right]. \quad (30)$$

It is noted that the associated retarded free phonon Green function, $D^{R(0)}_{\boldsymbol{q}}(t,t') = -2\sin\left[\omega_{\boldsymbol{q}ph}(t-t')\right]\theta(t-t')$, shows the contribution of incoherent phonon to the induced charge density of ionic core. Hence, the CP displacement function denoted as $Q_{\boldsymbol{q}}(\tau)$ turns out in proportion to $\Delta D^R_{\boldsymbol{q}}(t'+\tau,t') \equiv D^R_{\boldsymbol{q}}(t'+\tau,t') - D^{R(0)}_{\boldsymbol{q}}(t'+\tau,t')$; hereafter, it is understood that the external test potential is applied at $t'=0$. To be specific, this is given by

$$Q_{\boldsymbol{q}}(\tau) = -ie^{-i\omega_{\boldsymbol{q}ph}\tau}\left[\xi_{\boldsymbol{q}}(\tau,0)V^L_{\boldsymbol{q}phph}(\tau)V^{L\dagger}_{\boldsymbol{q}phph}(0) - 1\right] \times\theta(\tau) + (\mathrm{c.c.}), \quad (31)$$

aside from an unimportant proportional constant. By introducing real functions $\Theta_{\boldsymbol{q}}(\tau)$ and $A_{\boldsymbol{q}}(\tau)$ by

$$A_{\boldsymbol{q}}(\tau)e^{-i\Theta_{\boldsymbol{q}}(\tau)} = -2i\left[\xi_{\boldsymbol{q}}(\tau,0)V^L_{\boldsymbol{q}phph}(\tau)V^{L\dagger}_{\boldsymbol{q}phph}(0) - 1\right], \quad (32)$$

Eq. (31) is recast into

$$Q_{\boldsymbol{q}}(\tau) = A_{\boldsymbol{q}}(\tau)\cos\left[\omega_{\boldsymbol{q}ph}\tau + \Theta_{\boldsymbol{q}}(\tau)\right]. \quad (33)$$

Here, it is readily seen that

$$\Theta_{\boldsymbol{q}}(\tau) = \frac{\pi}{2} + \Phi_{\boldsymbol{q}}(\tau), \quad (34)$$

where

$$\Phi_{\boldsymbol{q}}(\tau) = -\arg\left[\xi_{\boldsymbol{q}}(\tau,0)V^L_{\boldsymbol{q}phph}(\tau)V^{L\dagger}_{\boldsymbol{q}phph}(0) - 1\right] \quad (35)$$

modulus $\pi$. In fact, $\xi_{\boldsymbol{q}}(\tau,0)$ can be set almost equal to unity, since both the energy shift of phonon given by $[\mathrm{Re}E_{\boldsymbol{q}ph}(\tau) - \omega_{\boldsymbol{q}ph}]$ and the phonon energy width of $\mathrm{Im}E_{\boldsymbol{q}ph}(\tau)$ are of the order of 1 meV, and thus, the phase integrals appearing in Eq. (30) are much smaller than $2\pi$ in the temporal region untill $\tau \approx 100$ fs concerned in this study; for the estimate of the energy shift, consult Fig.1(d) of the text. Incidentally, the CEP incorporated in Eq. (6) is ineffective under the rotating wave approximation stated above, as shown in Appendix B.

### Appendix A: Derivation of the Plasmon Operator $B^\dagger_{\boldsymbol{q}}$

To do this, first, the commutator given by

$$[\hat{H}_e + \hat{H}'(t), A^\dagger_{\boldsymbol{q}}(\boldsymbol{k}bb)] \approx \sum_{\boldsymbol{k}'b'} A^\dagger_{\boldsymbol{q}}(\boldsymbol{k}'b'b')Z_{\boldsymbol{q}}(\boldsymbol{k}'b'b',\boldsymbol{k}bb) + \Omega^{(R)}_{b\bar{b}}(t)A^\dagger_{\boldsymbol{q}}(\boldsymbol{k}b\bar{b}) - \Omega^{(R)}_{\bar{b}b}(t)A^\dagger_{\boldsymbol{q}}(\boldsymbol{k}\bar{b}b) \quad (\mathrm{A1})$$

is taken into account, where the first term of the right-hand side represents the contribution from intraband excitation with $Z_{\boldsymbol{q}}$ as the non-Hermitian matrix given by [1]

$$Z_{\boldsymbol{q}}(\boldsymbol{k}'b'b',\boldsymbol{k}bb) = \delta_{\boldsymbol{k}\boldsymbol{k}'}\delta_{bb'}\omega_{b'b'\boldsymbol{k}'\boldsymbol{q}} + V^{(C)}_{\boldsymbol{q}}(\rho_{bb\boldsymbol{k}} - \rho_{bb\boldsymbol{k}+\boldsymbol{q}}), \quad (\mathrm{A2})$$

and the second term represents the contribution from interband excitation. Here, four operator terms such as $a^\dagger_{b'\boldsymbol{k}'+\boldsymbol{q}}a_{b'\boldsymbol{k}'}a^\dagger_{b\boldsymbol{k}+\boldsymbol{q}}a_{b\boldsymbol{k}}$ are split into a product of the operator $A^\dagger_{\boldsymbol{q}}(\boldsymbol{k}'b'b')$ and a single-particle density matrix $\rho_{bb\boldsymbol{k}} \equiv \langle a^\dagger_{b\boldsymbol{k}}a_{b\boldsymbol{k}}\rangle$ by making a factorization approximation, $\omega_{bb\boldsymbol{k}\boldsymbol{q}} = \varepsilon^{(r)}_{b\boldsymbol{k}+\boldsymbol{q}} - \varepsilon^{(r)}_{b\boldsymbol{k}}$ with $\varepsilon^{(r)}_{b\boldsymbol{k}} = \varepsilon_{b\boldsymbol{k}} - \sum_{\boldsymbol{q}} V^{(C)}_{\boldsymbol{q}}\rho_{bb\boldsymbol{k}+\boldsymbol{q}}$ as renormalized $b$-band electron energy, and $\Omega^{(R)}_{b\bar{b}}(t)$ is given by Eq. (12).

Now, the left and right eigenvalue problems as $U^{L\dagger}_{\boldsymbol{q}}Z_{\boldsymbol{q}} = \mathcal{E}_{\boldsymbol{q}}U^{L\dagger}_{\boldsymbol{q}}$ and $Z_{\boldsymbol{q}}U^R_{\boldsymbol{q}} = U^R_{\boldsymbol{q}}\mathcal{E}_{\boldsymbol{q}}$, respectively, are solved, where $\mathcal{E}_{\boldsymbol{q}}$ is an eigenvalue, and $U^L_{\boldsymbol{q}}$ and $U^R_{\boldsymbol{q}}$ are the associated biorthogonal eigenvectors. In the long wave-length limit ($|\boldsymbol{q}| \to 0$), the non-vanishing solution arises just from the collective excitation mode of plasmon with $\mathcal{E}_{\boldsymbol{q}} = \omega_{\boldsymbol{q}pl}$, while the rest of intraband pair-excitation modes vanish. This procedure of introducing the plasmon mode somewhat differs from that developed in Ref. [2] in that just the contribution from intraband

excitation is incorporated here. The adiabatic plasma frequency $\omega_{\boldsymbol{q}pl}$ is given by

$$\omega_{\boldsymbol{q}pl} = \left[ V_{\boldsymbol{q}}^{(C)} \sum_{\boldsymbol{k}b} \rho_{bb\boldsymbol{k}} \nabla_{\boldsymbol{k}}^2 \varepsilon_{b\boldsymbol{k}}^{(r)} \right]^{\frac{1}{2}}. \quad \text{(A3)}$$

Further, both of $U_{\boldsymbol{q}}^{L\dagger}(\boldsymbol{k}bb)$ and $U_{\boldsymbol{q}}^{R}(\boldsymbol{k}bb)$ are readily obtained as

$$U_{\boldsymbol{q}}^{L\dagger}(\boldsymbol{k}bb) = N_{\boldsymbol{q}}^{L} V_{\boldsymbol{q}}^{(C)} g_{bb\boldsymbol{k}\boldsymbol{q}} (\rho_{bb\boldsymbol{k}} - \rho_{bb\boldsymbol{k}+\boldsymbol{q}}) \quad \text{(A4)}$$

and

$$U_{\boldsymbol{q}}^{R}(\boldsymbol{k}bb) = N_{\boldsymbol{q}}^{R} V_{\boldsymbol{q}}^{(C)} g_{bb\boldsymbol{k}\boldsymbol{q}}, \quad \text{(A5)}$$

respectively, where $g_{bb\boldsymbol{k}\boldsymbol{q}} = [\omega_{\boldsymbol{q}pl} - \omega_{bb\boldsymbol{k}\boldsymbol{q}}]^{-1}$. The normalization constants $N_{\boldsymbol{q}}^{L}$ and $N_{\boldsymbol{q}}^{R}$ are determined by the condition of $U_{\boldsymbol{q}}^{L\dagger} U_{\boldsymbol{q}}^{R} = 1$. From the above, the expression of $B_{\boldsymbol{q}}^{\dagger}$ is determined, as shown in Eq. (7).

### Appendix B: Eigenvalue Problem of the Matrix $\bar{Z}_{\boldsymbol{q}}$

Because of a relatively sparse form of $\bar{Z}_{\boldsymbol{q}}$, as seen in Eq. (20), both of a transcendental equation for determining a set of eigenvalues and the associated eigenvectors can be represented in analytic closed forms. The transcendental equation resulting from the eigenvalue equation of concern is given as

$$\prod_{j} (\bar{\omega}_{\boldsymbol{q}j} - E_{\boldsymbol{q}}) = \sum_{j \neq pl} M_{\boldsymbol{q}j} M'_{\boldsymbol{q}j} \prod_{j' \neq j, pl} (\bar{\omega}_{\boldsymbol{q}j'} - E_{\boldsymbol{q}}). \quad \text{(B1)}$$

To evaluate Eq. (33), just the expressions of $E_{\boldsymbol{q}ph}$ and the diagonal components of the associated left and right eigenvectors, $V_{\boldsymbol{q}phph}^{L\dagger}$ and $V_{\boldsymbol{q}phph}^{R}$, respectively, are necessary. These are given below. As regards this eigenvalue, Eq. (B1) is recast into

$$\begin{aligned} E_{\boldsymbol{q}ph} &= \bar{\omega}_{\boldsymbol{q}ph} - \frac{|M_{\boldsymbol{q}pl}|^2}{\bar{\omega}_{\boldsymbol{q}pl} - E_{\boldsymbol{q}ph}} \\ &\quad - \frac{\bar{\omega}_{\boldsymbol{q}ph} - E_{\boldsymbol{q}ph}}{\bar{\omega}_{\boldsymbol{q}pl} - E_{\boldsymbol{q}ph}} \sum_{\boldsymbol{k}b} \frac{M_{\boldsymbol{q}}(\boldsymbol{k}b\bar{b}) M'_{\boldsymbol{q}}(\boldsymbol{k}b\bar{b})}{\bar{\omega}_{b\bar{b}\boldsymbol{k}\boldsymbol{q}} - E_{\boldsymbol{q}ph}}, \end{aligned} \quad \text{(B2)}$$

and the eigenvectors are given by $V_{\boldsymbol{q}phph}^{L\dagger} = \bar{N}_{\boldsymbol{q}ph}^{L}$, and $V_{\boldsymbol{q}phph}^{R} = \bar{N}_{\boldsymbol{q}ph}^{R}$. Here, $\bar{N}_{\boldsymbol{q}ph}^{L}$ and $\bar{N}_{\boldsymbol{q}ph}^{R}$ are determined by the normalization condition of $V_{\boldsymbol{q}ph}^{L\dagger} V_{\boldsymbol{q}ph}^{R} = 1$, that is,

$$\begin{aligned} \left(\bar{N}_{\boldsymbol{q}ph}^{L} \bar{N}_{\boldsymbol{q}ph}^{R}\right)^{-1} &= 1 + \frac{(E_{\boldsymbol{q}ph} - \bar{\omega}_{\boldsymbol{q}ph})^2}{|M_{\boldsymbol{q}pl}|^2} \\ &\quad + \frac{(E_{\boldsymbol{q}ph} - \bar{\omega}_{\boldsymbol{q}ph})^2}{|M_{\boldsymbol{q}pl}|^2} \\ &\quad \times \sum_{\boldsymbol{k}b} \frac{M_{\boldsymbol{q}}(\boldsymbol{k}b\bar{b}) M'_{\boldsymbol{q}}(\boldsymbol{k}b\bar{b})}{E_{\boldsymbol{q}ph} - \bar{\omega}_{b\bar{b}\boldsymbol{k}\boldsymbol{q}}}. \end{aligned} \quad \text{(B3)}$$

Finally, it is remarked that the CEP of $\delta$ introduced in Eq. (6) has no contribution to the present CP dynamics under the rotating wave approximation. Actually, according to Eqs. (B2) and (B3), $M_{\boldsymbol{q}}(\boldsymbol{k}b\bar{b})$ and $M'_{\boldsymbol{q}}(\boldsymbol{k}b\bar{b})$ are always incorporated in the product form of $M_{\boldsymbol{q}}(\boldsymbol{k}b\bar{b}) M'_{\boldsymbol{q}}(\boldsymbol{k}b\bar{b})$, and the CEP term $\exp(i\bar{\delta}_{b\bar{b}})$ is factored out in $\bar{\rho}_{b\bar{b}k}$ of Eqs. (16) and (18). Therefore, it comes to the conclusion that the CEP is canceled exactly, as readily seen from Eqs. (16)-(18).


[1] H. Haug and S. W. Koch, *Quantum Theory of the Optical and Electronic Properties of Semiconductors, fifth ed.*, (World Scientific, Singapore, 2009) Chaps. 1 and 12.

[2] Y. Watanabe, K. Hino, M. Hase and N. Maeshima, Phys. Rev. B **95**, 014301 (2017).

[3] P. Meystre and M. Sargent III, *Elements of Quantum Optics, third ed.*, (Springer-Verlarg, Berlin, 1999) Chaps. 3 and 15.

[4] N. Moiseyev, *Non-Hermitian Quantum Mechanics*, (Cambridge, New York, 2011) Chaps. 7-9

[5] W. Schäfer and M. Wegener, *Semiconductor Optics and Transport Phenomena* (Springer-Verleg, Berlin, 2002) Chaps. 2, 10 and 11
